# Supplementary material for: Momentum distributions and numerical methods for strongly interacting one-dimensional spinor gases
Source: arXiv:1602.06816 ancillary file (2016-09-21)
Supplement: Supplementary file 1 [file exchange_coefficients.pdf]

# Exchange coefficients of harmonically trapped particles

Exchange coefficients in units of  $\hbar^2\omega^2l/g$ . Note the symmetry  $J_{N-i} = J_i$ .

| $N$ | $J_1$   | $J_2$   | $J_3$   | $J_4$   | ...     |         |         |         |         |         |
|-----|---------|---------|---------|---------|---------|---------|---------|---------|---------|---------|
| 2   | 0.7979  |         |         |         |         |         |         |         |         |         |
| 3   | 1.3464  |         |         |         |         |         |         |         |         |         |
| 4   | 1.7876  | 2.3465  |         |         |         |         |         |         |         |         |
| 5   | 2.1661  | 3.1772  |         |         |         |         |         |         |         |         |
| 6   | 2.5022  | 3.9021  | 4.3571  |         |         |         |         |         |         |         |
| 7   | 2.8074  | 4.5529  | 5.4003  |         |         |         |         |         |         |         |
| 8   | 3.0888  | 5.1481  | 6.345   | 6.7386  |         |         |         |         |         |         |
| 9   | 3.3511  | 5.6997  | 7.2143  | 7.959   |         |         |         |         |         |         |
| 10  | 3.5977  | 6.2159  | 8.0235  | 9.0879  | 9.4397  |         |         |         |         |         |
| 11  | 3.8311  | 6.7025  | 8.7833  | 10.1428 | 10.8152 |         |         |         |         |         |
| 12  | 4.0532  | 7.1641  | 9.5016  | 11.1364 | 12.1051 | 12.4261 |         |         |         |         |
| 13  | 4.2654  | 7.6041  | 10.1845 | 12.0781 | 13.3233 | 13.9412 |         |         |         |         |
| 14  | 4.4689  | 8.0252  | 10.8365 | 12.9751 | 14.4805 | 15.3756 | 15.6728 |         |         |         |
| 15  | 4.6648  | 8.4296  | 11.4615 | 13.833  | 15.5847 | 16.7409 | 17.3157 |         |         |         |
| 16  | 4.8537  | 8.8192  | 12.0625 | 14.6566 | 16.6426 | 18.046  | 18.8824 | 19.1602 |         |         |
| 17  | 5.0365  | 9.1954  | 12.642  | 15.4495 | 17.6594 | 19.2981 | 20.3822 | 20.9219 |         |         |
| 18  | 5.2136  | 9.5594  | 13.2022 | 16.2148 | 18.6394 | 20.503  | 21.8231 | 22.6109 | 22.8729 |         |
| 19  | 5.3855  | 9.9125  | 13.7447 | 16.9552 | 19.5863 | 21.6656 | 23.2112 | 24.2355 | 24.7458 |         |
| 20  | 5.5527  | 10.2554 | 14.2712 | 17.6729 | 20.5032 | 22.79   | 24.552  | 25.8023 | 26.5494 | 26.7978 |
| 21  | 5.7155  | 10.5891 | 14.783  | 18.3699 | 21.3927 | 23.8796 | 25.8499 | 27.3171 | 28.2905 | 28.7758 |
| 22  | 5.8743  | 10.9142 | 15.2811 | 19.0478 | 22.2571 | 24.9374 | 27.1086 | 28.7846 | 29.9753 | 30.6872 |
|     | 30.9241 |         |         |         |         |         |         |         |         |         |
| 23  | 6.0293  | 11.2313 | 15.7667 | 19.708  | 23.0982 | 25.966  | 28.3314 | 30.2089 | 31.6087 | 32.5383 |
|     | 33.0019 |         |         |         |         |         |         |         |         |         |
| 24  | 6.1808  | 11.541  | 16.2406 | 20.3519 | 23.918  | 26.9676 | 29.5212 | 31.5935 | 33.1952 | 34.3342 |
|     | 35.0156 | 35.2424 |         |         |         |         |         |         |         |         |
| 25  | 6.329   | 11.8438 | 16.7036 | 20.9806 | 24.7178 | 27.9443 | 30.6804 | 32.9414 | 34.7385 | 36.0797 |
|     | 36.9707 | 37.4154 |         |         |         |         |         |         |         |         |
| 26  | 6.4741  | 12.1401 | 17.1564 | 21.5951 | 25.4991 | 28.8976 | 31.8113 | 34.2555 | 36.2418 | 37.7786 |
|     | 38.8721 | 39.5266 | 39.7445 |         |         |         |         |         |         |         |
| 27  | 6.6163  | 12.4303 | 17.5997 | 22.1962 | 26.2631 | 29.8293 | 32.9158 | 35.5381 | 37.708  | 39.4344 |
|     | 40.7238 | 41.5809 | 42.0087 |         |         |         |         |         |         |         |
| 28  | 6.7558  | 12.7148 | 18.0339 | 22.7849 | 27.0108 | 30.7406 | 33.9955 | 36.7913 | 39.1398 | 41.0502 |
|     | 42.5294 | 43.5826 | 44.2132 | 44.4231 |         |         |         |         |         |         |
| 29  | 6.8927  | 12.9938 | 18.4597 | 23.3618 | 27.7432 | 31.6329 | 35.0522 | 38.0169 | 40.5393 | 42.6287 |
|     | 44.2923 | 45.5355 | 46.3623 | 46.7751 |         |         |         |         |         |         |
| 30  | 7.0272  | 13.2678 | 18.8775 | 23.9277 | 28.4611 | 32.5072 | 36.0871 | 39.2167 | 41.9086 | 44.1723 |
|     | 46.0152 | 47.443  | 48.46   | 49.0691 | 49.2719 |         |         |         |         |         |
| 31  | 7.1593  | 13.5369 | 19.2878 | 24.483  | 29.1655 | 33.3646 | 37.1015 | 40.3923 | 43.2496 | 45.6831 |
|     | 47.7006 | 49.308  | 50.5098 | 51.3092 | 51.7084 |         |         |         |         |         |

| $N$ | $J_1$   | $J_2$   | $J_3$   | $J_4$   | ...     |         |         |         |         |         |  |
|-----|---------|---------|---------|---------|---------|---------|---------|---------|---------|---------|--|
| 32  | 7.2892  | 13.8013 | 19.6908 | 25.0284 | 29.8571 | 34.206  | 38.0965 | 41.5449 | 44.5639 | 47.1632 |  |
|     | 49.351  | 51.1332 | 52.5147 | 53.4991 | 54.0887 | 54.2851 |         |         |         |         |  |
| 33  | 7.4171  | 14.0615 | 20.087  | 25.5644 | 30.5364 | 35.0322 | 39.0733 | 42.6759 | 45.8529 | 48.6144 |  |
|     | 50.9682 | 52.921  | 54.4775 | 55.6418 | 56.4164 | 56.8033 |         |         |         |         |  |
| 34  | 7.5429  | 14.3174 | 20.4768 | 26.0915 | 31.2041 | 35.844  | 40.0327 | 43.7865 | 47.1182 | 50.0381 |  |
|     | 52.5543 | 54.6735 | 56.4008 | 57.7402 | 58.6949 | 59.2669 | 59.4574 |         |         |         |  |
| 35  | 7.6668  | 14.5694 | 20.8603 | 26.6099 | 31.8608 | 36.6422 | 40.9756 | 44.8775 | 48.3608 | 51.4358 |  |
|     | 54.1109 | 56.3927 | 58.2867 | 59.7971 | 60.9271 | 61.6792 | 62.0548 |         |         |         |  |
| 36  | 7.7889  | 14.8175 | 21.238  | 27.1203 | 32.507  | 37.4274 | 41.9029 | 45.9501 | 49.582  | 52.809  |  |
|     | 55.6395 | 58.0804 | 60.1373 | 61.8146 | 63.1156 | 64.0432 | 64.599  | 64.7842 |         |         |  |
| 37  | 7.9093  | 15.0621 | 21.61   | 27.6229 | 33.1432 | 38.2001 | 42.8153 | 47.0051 | 50.7828 | 54.1588 |  |
|     | 57.1416 | 59.7383 | 61.9545 | 63.7949 | 65.263  | 66.3617 | 67.0931 | 67.4584 |         |         |  |
| 38  | 8.028   | 15.3031 | 21.9766 | 28.118  | 33.7697 | 38.961  | 43.7134 | 48.0434 | 51.9642 | 55.4863 |  |
|     | 58.6185 | 61.3678 | 63.74   | 65.7399 | 67.3713 | 68.6372 | 69.5398 | 70.0807 | 70.2609 |         |  |
| 39  | 8.145   | 15.5408 | 22.338  | 28.606  | 34.3872 | 39.7106 | 44.5978 | 49.0656 | 53.127  | 56.7927 |  |
|     | 60.0714 | 62.9703 | 65.4954 | 67.6515 | 69.4426 | 70.8719 | 71.9418 | 72.654  | 73.0099 |         |  |
| 40  | 8.2605  | 15.7753 | 22.6945 | 29.0872 | 34.9958 | 40.4493 | 45.4693 | 50.0725 | 54.2721 | 58.0788 |  |
|     | 61.5014 | 64.5471 | 67.2221 | 69.5313 | 71.4788 | 73.0679 | 74.3013 | 75.1809 | 75.7081 | 75.8838 |  |
| 41  | 8.3746  | 16.0068 | 23.0462 | 29.5619 | 35.596  | 41.1776 | 46.3283 | 51.0648 | 55.4002 | 59.3455 |  |
|     | 62.9094 | 66.0994 | 68.9215 | 71.3808 | 73.4815 | 75.2272 | 76.6206 | 77.6638 | 78.3584 | 78.7054 |  |
| 42  | 8.4872  | 16.2352 | 23.3933 | 30.0302 | 36.1881 | 41.8959 | 47.1753 | 52.043  | 56.5122 | 60.5937 |  |
|     | 64.2966 | 67.6282 | 70.5947 | 73.2013 | 75.4524 | 77.3515 | 78.9015 | 80.1048 | 80.9631 | 81.4775 |  |
| 43  | 81.6489 |         |         |         |         |         |         |         |         |         |  |
|     | 8.5984  | 16.4608 | 23.736  | 30.4925 | 36.7724 | 42.6047 | 48.0109 | 53.0077 | 57.6086 | 61.8242 |  |
| 44  | 65.6637 | 69.1345 | 72.2429 | 74.9942 | 77.3928 | 79.4423 | 81.1459 | 82.506  | 83.5244 | 84.2026 |  |
|     | 84.5415 |         |         |         |         |         |         |         |         |         |  |
| 44  | 8.7083  | 16.6837 | 24.0744 | 30.949  | 37.3492 | 43.3042 | 48.8354 | 53.9595 | 58.69   | 63.0377 |  |
|     | 67.0116 | 70.6193 | 73.8672 | 76.7606 | 79.304  | 81.5013 | 83.3555 | 84.8692 | 86.0445 | 86.883  |  |
| 45  | 87.3856 | 87.553  |         |         |         |         |         |         |         |         |  |
|     | 8.8169  | 16.9039 | 24.4088 | 31.3998 | 37.9188 | 43.9948 | 49.6492 | 54.8989 | 59.7571 | 64.2348 |  |
| 46  | 68.341  | 72.0835 | 75.4686 | 78.5017 | 81.1874 | 83.5297 | 85.5317 | 87.1962 | 88.5253 | 89.5206 |  |
|     | 90.1835 | 90.5148 |         |         |         |         |         |         |         |         |  |
| 46  | 8.9242  | 17.1215 | 24.7392 | 31.8452 | 38.4815 | 44.6769 | 50.4529 | 55.8262 | 60.8103 | 65.4161 |  |
|     | 69.6528 | 73.5279 | 77.0479 | 80.2185 | 83.0442 | 85.5289 | 87.6761 | 89.4885 | 90.9684 | 92.1176 |  |
| 47  | 92.9375 | 93.4291 | 93.5929 |         |         |         |         |         |         |         |  |
|     | 9.0304  | 17.3367 | 25.0657 | 32.2854 | 39.0375 | 45.3507 | 51.2466 | 56.742  | 61.8503 | 66.5823 |  |
| 48  | 70.9474 | 74.9532 | 78.6062 | 81.9119 | 84.8752 | 87.5001 | 89.7899 | 91.7477 | 93.3756 | 94.6757 |  |
|     | 95.6495 | 96.2981 | 96.6222 |         |         |         |         |         |         |         |  |
| 48  | 9.1354  | 17.5495 | 25.3886 | 32.7206 | 39.5869 | 46.0166 | 52.0309 | 57.6467 | 62.8774 | 67.734  |  |
|     | 72.2257 | 76.3602 | 80.1441 | 83.583  | 86.6817 | 89.4444 | 91.8745 | 93.975  | 95.7483 | 97.1966 |  |
| 49  | 98.3214 | 99.1239 | 99.6051 | 99.7654 |         |         |         |         |         |         |  |
|     | 9.2393  | 17.7599 | 25.7079 | 33.1508 | 40.1302 | 46.6747 | 52.806  | 58.5406 | 63.8922 | 68.8716 |  |
| 49  | 73.4881 | 77.7495 | 81.6624 | 85.2324 | 88.4645 | 91.3628 | 93.9309 | 96.1717 | 98.088  | 99.6817 |  |
|     | 100.955 | 101.908 | 102.544 | 102.861 |         |         |         |         |         |         |  |

| $N$ | $J_1$   | $J_2$   | $J_3$   | $J_4$   | ...     |         |         |         |         |         |  |
|-----|---------|---------|---------|---------|---------|---------|---------|---------|---------|---------|--|
| 50  | 9.3421  | 17.9682 | 26.0238 | 33.5764 | 40.6673 | 47.3255 | 53.5722 | 59.4242 | 64.895  | 69.9956 |  |
|     | 74.7352 | 79.1217 | 83.1618 | 86.8611 | 90.2245 | 93.2563 | 95.9602 | 98.3392 | 100.396 | 102.133 |  |
|     | 103.551 | 104.653 | 105.439 | 105.911 | 106.068 |         |         |         |         |         |  |
| 51  | 9.4438  | 18.1742 | 26.3363 | 33.9973 | 41.1987 | 47.969  | 54.3298 | 60.2977 | 65.8863 | 71.1065 |  |
|     | 75.9676 | 80.4776 | 84.643  | 88.4697 | 91.9626 | 95.1259 | 97.9635 | 100.478 | 102.673 | 104.551 |  |
|     | 106.112 | 107.36  | 108.295 | 108.917 | 109.228 |         |         |         |         |         |  |
| 52  | 9.5446  | 18.3782 | 26.6455 | 34.4138 | 41.7243 | 48.6056 | 55.0791 | 61.1615 | 66.8664 | 72.2047 |  |
|     | 77.1858 | 81.8176 | 86.1067 | 90.059  | 93.6795 | 96.9724 | 99.9417 | 102.59  | 104.922 | 106.937 |  |
|     | 108.64  | 110.03  | 111.111 | 111.881 | 112.344 | 112.498 |         |         |         |         |  |
| 53  | 9.6443  | 18.5801 | 26.9517 | 34.8261 | 42.2444 | 49.2354 | 55.8204 | 62.016  | 67.8357 | 73.2907 |  |
|     | 78.3903 | 83.1422 | 87.5534 | 91.6296 | 95.3759 | 98.7967 | 101.896 | 104.676 | 107.141 | 109.293 |  |
|     | 111.134 | 112.665 | 113.889 | 114.806 | 115.416 | 115.722 |         |         |         |         |  |
| 54  | 9.7431  | 18.78   | 27.2547 | 35.2341 | 42.7593 | 49.8587 | 56.5538 | 62.8613 | 68.7946 | 74.3649 |  |
|     | 79.5814 | 84.4521 | 88.9837 | 93.1822 | 97.0527 | 100.599 | 103.826 | 106.737 | 109.334 | 111.62  |  |
|     | 113.597 | 115.267 | 116.631 | 117.691 | 118.448 | 118.901 | 119.052 |         |         |         |  |
| 55  | 9.8409  | 18.978  | 27.5548 | 35.6381 | 43.2689 | 50.4756 | 57.2797 | 63.6978 | 69.7433 | 75.4275 |  |
|     | 80.7596 | 85.7475 | 90.3982 | 94.7174 | 98.7103 | 102.381 | 105.735 | 108.773 | 111.5   | 113.918 |  |
|     | 116.03  | 117.836 | 119.339 | 120.54  | 121.439 | 122.039 | 122.338 |         |         |         |  |
| 56  | 9.9378  | 19.1741 | 27.852  | 36.0382 | 43.7735 | 51.0864 | 57.9983 | 64.5257 | 70.6823 | 76.479  |  |
|     | 81.9253 | 87.0291 | 91.7972 | 96.2356 | 100.35  | 104.143 | 107.621 | 110.786 | 113.641 | 116.189 |  |
|     | 118.433 | 120.373 | 122.013 | 123.352 | 124.393 | 125.136 | 125.581 | 125.73  |         |         |  |
| 57  | 10.0338 | 19.3684 | 28.1464 | 36.4345 | 44.2733 | 51.6912 | 58.7097 | 65.3454 | 71.6117 | 77.5197 |  |
|     | 83.0789 | 88.2972 | 93.1814 | 97.7376 | 101.971 | 105.886 | 109.486 | 112.776 | 115.758 | 118.434 |  |
|     | 120.808 | 122.881 | 124.654 | 126.13  | 127.31  | 128.194 | 128.782 | 129.077 |         |         |  |
| 58  | 10.129  | 19.5609 | 28.4381 | 36.827  | 44.7682 | 52.2902 | 59.4143 | 66.157  | 72.5318 | 78.55   |  |
|     | 84.2207 | 89.5522 | 94.5512 | 99.2236 | 103.575 | 107.609 | 111.331 | 114.744 | 117.85  | 120.653 |  |
|     | 123.156 | 125.359 | 127.265 | 128.875 | 130.191 | 131.214 | 131.944 | 132.381 | 132.527 |         |  |
| 59  | 10.2233 | 19.7517 | 28.7272 | 37.2159 | 45.2586 | 52.8836 | 60.1121 | 66.9607 | 73.443  | 79.57   |  |
|     | 85.3512 | 90.7945 | 95.9069 | 100.694 | 105.162 | 109.315 | 113.156 | 116.69  | 119.92  | 122.848 |  |
|     | 125.477 | 127.809 | 129.845 | 131.588 | 133.039 | 134.198 | 135.066 | 135.645 | 135.934 |         |  |
| 60  | 10.3169 | 19.9408 | 29.0137 | 37.6014 | 45.7445 | 53.4714 | 60.8033 | 67.7569 | 74.3454 | 80.5802 |  |
|     | 86.4706 | 92.0246 | 97.2491 | 102.15  | 106.733 | 111.002 | 114.962 | 118.616 | 121.967 | 125.019 |  |
|     | 127.773 | 130.231 | 132.396 | 134.27  | 135.853 | 137.146 | 138.152 | 138.869 | 139.299 | 139.443 |  |
