# Supplementary material for: Momentum distributions and numerical methods for strongly interacting one-dimensional spinor gases
Source: arXiv:1602.06816 ancillary file (2016-09-21)
Supplement: Supplementary file 2 [file one_body_density_matrix.pdf]

# An efficient formula for the one-body density matrix elements

Frank Deuretzbacher

## 1 Spin momentum distribution

probability that a particle has momentum  $k = p/\hbar$  and magnetization  $m$

$$\hat{\rho}_m(k) \equiv \sum_{i=1}^N |k\rangle_i \langle k|_i |m\rangle_i \langle m|_i \quad (1)$$

$|k\rangle$  in position space (i: imaginary unit)

$$|k\rangle = \int_{-\infty}^{\infty} dz |z\rangle \langle z|k\rangle = \frac{1}{\sqrt{2\pi}} \int_{-\infty}^{\infty} dz |z\rangle e^{\mathrm{i}kz} \quad (2)$$

spin-independent momentum distribution of  $i$ th particle

$$\hat{\rho}^{(i)}(k) \equiv |k\rangle_i \langle k|_i = \frac{1}{2\pi} \int_{-\infty}^{\infty} \int_{-\infty}^{\infty} dz dz' e^{\mathrm{i}k(z-z')} |z\rangle_i \langle z'|_i \quad (3)$$

probability that  $i$ th spin has magnetization  $m$

$$\hat{\rho}_m^{(i)} \equiv |m\rangle_i \langle m|_i = \sum_{m_1, \dots, m_N} \delta_{m, m_i} |m_1, \dots, m_N\rangle \langle m_1, \dots, m_N| \quad (4)$$

therefore

$$\hat{\rho}_m(k) = \sum_{i=1}^N \hat{\rho}^{(i)}(k) \hat{\rho}_m^{(i)} \quad (5)$$

spin-independent one-body density matrix of  $i$ th particle

$$\begin{aligned} \hat{\rho}^{(i)}(z, z') &\equiv |z\rangle_i \langle z'|_i = \int dz_1 \cdots dz_{i-1} dz_{i+1} \cdots dz_N |z_1, \dots, z_{i-1}, z, z_{i+1}, \dots, z_N\rangle \\ &\quad \times \langle z_1, \dots, z_{i-1}, z', z_{i+1}, \dots, z_N| \end{aligned} \quad (6)$$

relationship between momentum distribution and one-body density matrix of  $i$ th particle

$$\hat{\rho}^{(i)}(k) = \frac{1}{2\pi} \int_{-\infty}^{\infty} \int_{-\infty}^{\infty} dz dz' e^{\mathrm{i}k(z-z')} \hat{\rho}^{(i)}(z, z') \quad (7)$$

therefore

$$\hat{\rho}_m(k) = \sum_{i=1}^N \frac{1}{2\pi} \int_{-\infty}^{\infty} \int_{-\infty}^{\infty} dz dz' e^{ik(z-z')} \hat{\rho}^{(i)}(z, z') \hat{\rho}_m^{(i)} \quad (8)$$

spin momentum distribution of state  $W_{\pm}|\chi\rangle \equiv \sqrt{N!}S_{\pm}|\text{id}\rangle|\chi\rangle$

$$\begin{aligned} \rho_m(k) &\equiv \langle \chi | W_{\pm}^{\dagger} \hat{\rho}_m(k) W_{\pm} | \chi \rangle = \sum_P (\pm 1)^P \langle \chi | \langle \text{id} | \hat{\rho}_m(k) | P \rangle (P | \chi) \rangle \\ &= \sum_i \sum_P (\pm 1)^P \frac{1}{2\pi} \int_{-\infty}^{\infty} \int_{-\infty}^{\infty} dz dz' e^{ik(z-z')} \langle \text{id} | \hat{\rho}^{(i)}(z, z') | P \rangle \langle \chi | \hat{\rho}_m^{(i)}(P | \chi) \rangle \end{aligned} \quad (9)$$

We show in Sec. 3 that only the matrix elements  $\rho^{(i,j)}(z, z') \equiv \langle \text{id} | \hat{\rho}^{(i)}(z, z') | P_{(i,\dots,j)} \rangle$  are nonzero, where the loop-permutation operator  $P_{(i,\dots,j)}$  is defined by Eq. (35). Therefore, we obtain

$$\rho_m(k) = \sum_{i=1}^N \sum_{j=1}^N (\pm 1)^{i+j} \frac{1}{2\pi} \int_{-\infty}^{\infty} \int_{-\infty}^{\infty} dz dz' e^{ik(z-z')} \rho^{(i,j)}(z, z') \langle \chi | \hat{\rho}_m^{(i)}(P_{(i,\dots,j)} | \chi) \rangle. \quad (10)$$

Here, we used

$$(\pm 1)^{P_{(i,\dots,j)}} = (\pm 1)^{P_{(i,i+1)}P_{(i+1,i+2)}\dots P_{(j-2,j-1)}P_{(j-1,j)}} = (\pm 1)^{j-i} = (\pm 1)^{i+j} \quad (11)$$

for  $i < j$  and

$$(\pm 1)^{P_{(i,\dots,j)}} = (\pm 1)^{P_{(i,i-1)}P_{(i-1,i-2)}\dots P_{(j+2,j+1)}P_{(j+1,j)}} = (\pm 1)^{i-j} = (\pm 1)^{i+j} \quad (12)$$

for  $i > j$ , respectively.

## 2 Spin occupation number distribution

probability that a particle is in energy eigenstate  $n$  and has magnetization  $m$

$$\hat{\rho}_m(n) \equiv \sum_{i=1}^N |n\rangle_i \langle n|_i |m\rangle_i \langle m|_i \quad (13)$$

$|n\rangle$  in position space

$$|n\rangle = \int_{-\infty}^{\infty} dz |z\rangle \langle z|n\rangle = \frac{1}{\sqrt{2\pi}} \int_{-\infty}^{\infty} dz |z\rangle \phi_n(z) \quad (14)$$

spin-independent occupation number distribution of  $i$ th particle

$$\hat{\rho}^{(i)}(n) \equiv |n\rangle_i \langle n|_i = \int_{-\infty}^{\infty} \int_{-\infty}^{\infty} dz dz' \phi_n(z) \phi_n^*(z') |z\rangle_i \langle z'|_i \quad (15)$$

probability that  $i$ th spin has magnetization  $m$

$$\hat{\rho}_m^{(i)} \equiv |m\rangle_i \langle m|_i = \sum_{m_1, \dots, m_N} \delta_{m, m_i} |m_1, \dots, m_N\rangle \langle m_1, \dots, m_N| \quad (16)$$

therefore

$$\hat{\rho}_m(n) = \sum_{i=1}^N \hat{\rho}^{(i)}(n) \hat{\rho}_m^{(i)} \quad (17)$$

spin-independent one-body density matrix of  $i$ th particle

$$\begin{aligned} \hat{\rho}^{(i)}(z, z') &\equiv |z\rangle_i \langle z'|_i = \int dz_1 \cdots dz_{i-1} dz_{i+1} \cdots dz_N |z_1, \dots, z_{i-1}, z, z_{i+1}, \dots, z_N\rangle \\ &\quad \times \langle z_1, \dots, z_{i-1}, z', z_{i+1}, \dots, z_N| \end{aligned} \quad (18)$$

relationship between occupation number distribution and one-body density matrix of  $i$ th particle

$$\hat{\rho}^{(i)}(n) = \int_{-\infty}^{\infty} \int_{-\infty}^{\infty} dz dz' \phi_n(z) \phi_n^*(z') \hat{\rho}^{(i)}(z, z') \quad (19)$$

therefore

$$\hat{\rho}_m(n) = \sum_{i=1}^N \int_{-\infty}^{\infty} \int_{-\infty}^{\infty} dz dz' \phi_n(z) \phi_n^*(z') \hat{\rho}^{(i)}(z, z') \hat{\rho}_m^{(i)} \quad (20)$$

spin occupation number distribution of state  $W_{\pm}|\chi\rangle \equiv \sqrt{N!} S_{\pm} |\text{id}\rangle |\chi\rangle$

$$\begin{aligned} \rho_m(n) &\equiv \langle \chi | W_{\pm}^{\dagger} \hat{\rho}_m(n) W_{\pm} | \chi \rangle = \sum_P (\pm 1)^P \langle \chi | \langle \text{id} | \hat{\rho}_m(n) | P \rangle (P | \chi \rangle) \\ &= \sum_i \sum_P (\pm 1)^P \int_{-\infty}^{\infty} \int_{-\infty}^{\infty} dz dz' \phi_n(z) \phi_n^*(z') \langle \text{id} | \hat{\rho}^{(i)}(z, z') | P \rangle \langle \chi | \hat{\rho}_m^{(i)}(P | \chi \rangle) \end{aligned} \quad (21)$$

We show in Sec. 3 that only the matrix elements  $\rho^{(i,j)}(z, z') \equiv \langle \text{id} | \hat{\rho}^{(i)}(z, z') | P_{(i, \dots, j)} \rangle$  are nonzero, where the loop-permutation operator  $P_{(i, \dots, j)}$  is defined by Eq. (35). Therefore, we obtain

$$\rho_m(n) = \sum_{i=1}^N \sum_{j=1}^N (\pm 1)^{i+j} \int_{-\infty}^{\infty} \int_{-\infty}^{\infty} dz dz' \phi_n(z) \phi_n^*(z') \rho^{(i,j)}(z, z') \langle \chi | \hat{\rho}_m^{(i)}(P_{(i, \dots, j)} | \chi \rangle). \quad (22)$$

### 3 One-body density matrix elements

$$\begin{aligned} \langle \text{id} | \hat{\rho}^{(i)}(z, z') | P \rangle &= \langle \text{id} | z \rangle_i \langle z' |_i | P \rangle = \int dz_1 \cdots dz_{i-1} dz_{i+1} \cdots dz_N \\ &\quad \times \langle \text{id} | z_1, \dots, z_{i-1}, z, z_{i+1}, \dots, z_N \rangle \langle z_1, \dots, z_{i-1}, z', z_{i+1}, \dots, z_N | P \rangle \end{aligned} \quad (23)$$

$$\begin{aligned} &= N! \int dz_1 \cdots dz_{i-1} dz_{i+1} \cdots dz_N \left[ \theta(z_1, \dots, z_N) \left| \psi_F(z_1, \dots, z_N) \right| \right]_{z_i=z} \\ &\quad \times \left[ \theta(z_{P(1)}, \dots, z_{P(N)}) \left| \psi_F(z_1, \dots, z_N) \right| \right]_{z_i=z'} \end{aligned} \quad (24)$$

For which permutations  $P$  is this integral nonzero? Consider the example  $N = 5, i = 2$ . Only the following 5 integrals are nonzero:

$$\begin{aligned} \langle \text{id} | \hat{\rho}^{(2)}(z, z') | P_{(2,1)} \rangle &= 5! \int dz_1 dz_3 dz_4 dz_5 \theta(z_1, z, z_3, z_4, z_5) \theta(z', z_1, z_3, z_4, z_5) \\ &\quad \times |\psi_F(z_1, z, z_3, z_4, z_5) \psi_F(z_1, z', z_3, z_4, z_5)| \end{aligned} \quad (25)$$

$$\begin{aligned} &= 5! \theta(z', z) \int_{z' < z_1 < z < z_3 < z_4 < z_5} dz_1 dz_3 dz_4 dz_5 |\psi_F(z_1, z, z_3, z_4, z_5)| \\ &\quad \times |\psi_F(z_1, z', z_3, z_4, z_5)|, \end{aligned} \quad (26)$$

$$\begin{aligned} \langle \text{id} | \hat{\rho}^{(2)}(z, z') | \text{id} \rangle &= 5! \int dz_1 dz_3 dz_4 dz_5 \theta(z_1, z, z_3, z_4, z_5) \theta(z_1, z', z_3, z_4, z_5) \\ &\quad \times |\psi_F(z_1, z, z_3, z_4, z_5) \psi_F(z_1, z', z_3, z_4, z_5)| \end{aligned} \quad (27)$$

$$\begin{aligned} &= 5! \int_{z_1 < z, z' < z_3 < z_4 < z_5} dz_1 dz_3 dz_4 dz_5 |\psi_F(z_1, z, z_3, z_4, z_5)| \\ &\quad \times |\psi_F(z_1, z', z_3, z_4, z_5)|, \end{aligned} \quad (28)$$

$$\begin{aligned} \langle \text{id} | \hat{\rho}^{(2)}(z, z') | P_{(2,3)} \rangle &= 5! \int dz_1 dz_3 dz_4 dz_5 \theta(z_1, z, z_3, z_4, z_5) \theta(z_1, z_3, z', z_4, z_5) \\ &\quad \times |\psi_F(z_1, z, z_3, z_4, z_5) \psi_F(z_1, z', z_3, z_4, z_5)| \end{aligned} \quad (29)$$

$$\begin{aligned} &= 5! \theta(z, z') \int_{z_1 < z < z_3 < z' < z_4 < z_5} dz_1 dz_3 dz_4 dz_5 |\psi_F(z_1, z, z_3, z_4, z_5)| \\ &\quad \times |\psi_F(z_1, z', z_3, z_4, z_5)|, \end{aligned} \quad (30)$$

$$\begin{aligned} \langle \text{id} | \hat{\rho}^{(2)}(z, z') | P_{(2,3,4)} \rangle &= 5! \int dz_1 dz_3 dz_4 dz_5 \theta(z_1, z, z_3, z_4, z_5) \theta(z_1, z_3, z_4, z', z_5) \\ &\quad \times |\psi_F(z_1, z, z_3, z_4, z_5) \psi_F(z_1, z', z_3, z_4, z_5)| \end{aligned} \quad (31)$$

$$\begin{aligned} &= 5! \theta(z, z') \int_{z_1 < z < z_3 < z_4 < z' < z_5} dz_1 dz_3 dz_4 dz_5 |\psi_F(z_1, z, z_3, z_4, z_5)| \\ &\quad \times |\psi_F(z_1, z', z_3, z_4, z_5)|, \end{aligned} \quad (32)$$

$$\begin{aligned} \langle \text{id} | \hat{\rho}^{(2)}(z, z') | P_{(2,3,4,5)} \rangle &= 5! \int dz_1 dz_3 dz_4 dz_5 \theta(z_1, z, z_3, z_4, z_5) \theta(z_1, z_3, z_4, z_5, z') \\ &\quad \times |\psi_F(z_1, z, z_3, z_4, z_5) \psi_F(z_1, z', z_3, z_4, z_5)| \end{aligned} \quad (33)$$

$$\begin{aligned} &= 5! \theta(z, z') \int_{z_1 < z < z_3 < z_4 < z_5 < z'} dz_1 dz_3 dz_4 dz_5 |\psi_F(z_1, z, z_3, z_4, z_5)| \\ &\quad \times |\psi_F(z_1, z', z_3, z_4, z_5)|. \end{aligned} \quad (34)$$

We conclude that, in the general case, the integral is only nonzero for the loop permutations  $P_{(i,i-1,\dots,j+1,j)}$  for  $i > j$ ,  $\text{id}$ , and  $P_{(i,i+1,\dots,j-1,j)}$  for  $i < j$ . Here we used the cycle notation, i.e.,  $P_{\alpha,\beta,\gamma}$  maps  $\alpha$  on  $\beta$ ,  $\beta$  on  $\gamma$ , and  $\gamma$  on  $\alpha$ . We abbreviate the loop permutations by the symbol

$$P_{(i,\dots,j)} \equiv \begin{cases} P_{(i,i-1,\dots,j+1,j)} & \text{for } i > j \\ \text{id} & \text{for } i = j \\ P_{(i,i+1,\dots,j-1,j)} & \text{for } i < j. \end{cases} \quad (35)$$

We define the nonzero matrix elements of the one-body density matrix by

$$\rho^{(i,j)}(z, z') \equiv \langle \text{id} | \hat{\rho}^{(i)}(z, z') | P_{(i,\dots,j)} \rangle. \quad (36)$$

We will see later that  $(i, j)$  corresponds to the position in the  $(z, z')$  plane. The previous example showed that for  $i > j$ :

$$\begin{aligned} \rho^{(i,j)}(z, z') &= N! \theta(z', z) \int_{z_1 < \dots < z_{j-1} < z' < z_j < \dots < z_{i-1} < z < z_{i+1} < \dots < z_N} dz_1 \dots dz_{i-1} dz_{i+1} \dots dz_N \\ &\times \left| \psi_F(z_1, \dots, z_{i-1}, z, z_{i+1}, \dots, z_N) \psi_F(z_1, \dots, z_{i-1}, z', z_{i+1}, \dots, z_N) \right|, \end{aligned} \quad (37)$$

for  $i = j$ :

$$\begin{aligned} \rho^{(i,i)}(z, z') &= N! \int_{z_1 < \dots < z_{i-1} < z, z' < z_{i+1} < \dots < z_N} dz_1 \dots dz_{i-1} dz_{i+1} \dots dz_N \\ &\times \left| \psi_F(z_1, \dots, z_{i-1}, z, z_{i+1}, \dots, z_N) \psi_F(z_1, \dots, z_{i-1}, z', z_{i+1}, \dots, z_N) \right|, \end{aligned} \quad (38)$$

and for  $i < j$ :

$$\begin{aligned} \rho^{(i,j)}(z, z') &= N! \theta(z, z') \int_{z_1 < \dots < z_{i-1} < z < z_{i+1} < \dots < z_j < z' < z_{j+1} < \dots < z_N} dz_1 \dots dz_{i-1} dz_{i+1} \dots dz_N \\ &\times \left| \psi_F(z_1, \dots, z_{i-1}, z, z_{i+1}, \dots, z_N) \psi_F(z_1, \dots, z_{i-1}, z', z_{i+1}, \dots, z_N) \right|. \end{aligned} \quad (39)$$

The following derivation is restricted to the case  $i < j$ . The other cases will be discussed subsequently. First, we would like to get rid of the absolute value. Consider the product

$$\begin{aligned} &\theta(z_1, \dots, z_{i-1}, z, z_{i+1}, \dots, z_N) \theta(z_1, \dots, z_{i-1}, z_{i+1}, \dots, z_j, z', z_{j+1}, \dots, z_N) \\ &\times \left| \psi_F(z_1, \dots, z_{i-1}, z, z_{i+1}, \dots, z_N) \psi_F(z_1, \dots, z_{i-1}, z', z_{i+1}, \dots, z_N) \right|. \end{aligned} \quad (40)$$

Due to the antisymmetry of  $\psi_F$  we may exchange the arguments of the second  $\psi_F$  to obtain

$$\begin{aligned} &\theta(z_1, \dots, z_{i-1}, z, z_{i+1}, \dots, z_N) \theta(z_1, \dots, z_{i-1}, z_{i+1}, \dots, z_j, z', z_{j+1}, \dots, z_N) \\ &\times \left| \psi_F(z_1, \dots, z_{i-1}, z, z_{i+1}, \dots, z_N) \psi_F(z_1, \dots, z_{i-1}, z', z_{i+1}, \dots, z_N) \right| \\ &= \theta(z_1, \dots, z_{i-1}, z, z_{i+1}, \dots, z_N) \theta(z_1, \dots, z_{i-1}, z_{i+1}, \dots, z_j, z', z_{j+1}, \dots, z_N) \\ &\times \left| \psi_F(z_1, \dots, z_{i-1}, z, z_{i+1}, \dots, z_N) \psi_F(z_1, \dots, z_{i-1}, z_{i+1}, \dots, z_j, z', z_{j+1}, \dots, z_N) \right|. \end{aligned} \quad (41)$$

Both  $\psi_F$  live now in the same sector of the configuration space. Therefore, we may omit the absolute value and obtain

$$\begin{aligned} & \theta(z_1, \dots, z_{i-1}, z, z_{i+1}, \dots, z_N) \theta(z_1, \dots, z_{i-1}, z_{i+1}, \dots, z_j, z', z_{j+1}, \dots, z_N) \\ & \times \left| \psi_F(z_1, \dots, z_{i-1}, z, z_{i+1}, \dots, z_N) \psi_F(z_1, \dots, z_{i-1}, z', z_{i+1}, \dots, z_N) \right| \\ & = \theta(z_1, \dots, z_{i-1}, z, z_{i+1}, \dots, z_N) \theta(z_1, \dots, z_{i-1}, z_{i+1}, \dots, z_j, z', z_{j+1}, \dots, z_N) \\ & \times \psi_F(z_1, \dots, z_{i-1}, z, z_{i+1}, \dots, z_N) \psi_F(z_1, \dots, z_{i-1}, z_{i+1}, \dots, z_j, z', z_{j+1}, \dots, z_N). \end{aligned} \quad (42)$$

Finally, we move  $z'$  back to the  $i$ th position in the second  $\psi_F$ . We need  $j - i$  transpositions of  $z'$  with its left nearest neighbors to achieve this. Due to the antisymmetry of  $\psi_F$  we have to multiply with the factor  $(-1)^{j-i} = (-1)^{i+j}$  and obtain

$$\begin{aligned} & \theta(z_1, \dots, z_{i-1}, z, z_{i+1}, \dots, z_N) \theta(z_1, \dots, z_{i-1}, z_{i+1}, \dots, z_j, z', z_{j+1}, \dots, z_N) \\ & \times \left| \psi_F(z_1, \dots, z_{i-1}, z, z_{i+1}, \dots, z_N) \psi_F(z_1, \dots, z_{i-1}, z', z_{i+1}, \dots, z_N) \right| \\ & = \theta(z_1, \dots, z_{i-1}, z, z_{i+1}, \dots, z_N) \theta(z_1, \dots, z_{i-1}, z_{i+1}, \dots, z_j, z', z_{j+1}, \dots, z_N) \\ & \times (-1)^{i+j} \psi_F(z_1, \dots, z_{i-1}, z, z_{i+1}, \dots, z_N) \psi_F(z_1, \dots, z_{i-1}, z', z_{i+1}, \dots, z_N). \end{aligned} \quad (43)$$

Therefore

$$\begin{aligned} \rho^{(i,j)}(z, z') &= (-1)^{i+j} N! \theta(z, z') \int_{z_1 < \dots < z_{i-1} < z < z_{i+1} < \dots < z_j < z' < z_{j+1} < \dots < z_N} dz_1 \dots dz_{i-1} dz_{i+1} \dots dz_N \\ &\times \psi_F(z_1, \dots, z_{i-1}, z, z_{i+1}, \dots, z_N) \psi_F(z_1, \dots, z_{i-1}, z', z_{i+1}, \dots, z_N). \end{aligned} \quad (44)$$

The integrand is symmetric under permutations of  $z_1, \dots, z_{i-1}, z_{i+1}, \dots, z_j$ , and  $z_{j+1}, \dots, z_N$ . Therefore

$$\begin{aligned} \rho^{(i,j)}(z, z') &= (-1)^{i+j} \theta(z, z') \frac{N!}{(i-1)!(j-i)!(N-j)!} \\ &\times \int_{z_1, \dots, z_{i-1} < z < z_{i+1}, \dots, z_j < z' < z_{j+1}, \dots, z_N} dz_1 \dots dz_{i-1} dz_{i+1} \dots dz_N \\ &\times \psi_F(z_1, \dots, z_{i-1}, z, z_{i+1}, \dots, z_N) \psi_F(z_1, \dots, z_{i-1}, z', z_{i+1}, \dots, z_N). \end{aligned} \quad (45)$$

use

$$\psi_F(z_1, \dots, z_N) = \frac{1}{\sqrt{N!}} \sum_P (-1)^P \prod_{i=1}^N \phi_{P(i)}(z_i) \quad (46)$$

define 1d integrals

$$A_{i,j}(z) \equiv \int_{-\infty}^z dx \phi_i(x) \phi_j(x) = \delta_{i,j} - B_{i,j}(z) \quad (47)$$

$$B_{i,j}(z) \equiv \int_z^{\infty} dx \phi_i(x) \phi_j(x) \quad (48)$$

$$C_{i,j}(z, z') \equiv \int_z^{z'} dx \phi_i(x) \phi_j(x) = B_{i,j}(z) - B_{i,j}(z') \quad (49)$$

then

$$\begin{aligned} \rho^{(i,j)}(z, z') &= \frac{(-1)^{i+j}\theta(z, z')}{(i-1)!(j-i)!(N-j)!} \sum_{P, P'} (-1)^P (-1)^{P'} A_{P(1), P'(1)}(z) \cdots A_{P(i-1), P'(i-1)}(z) \\ &\quad \times \phi_{P(i)}(z) \phi_{P'(i)}(z') C_{P(i+1), P'(i+1)}(z, z') \cdots C_{P(j), P'(j)}(z, z') \\ &\quad \times B_{P(j+1), P'(j+1)}(z') \cdots B_{P(N), P'(N)}(z') \end{aligned} \quad (50)$$

introduce  $P''$  defined by  $P' = P'' \circ P$ , sum over  $P, P''$

$$\begin{aligned} \rho^{(i,j)}(z, z') &= \frac{(-1)^{i+j}\theta(z, z')}{(i-1)!(j-i)!(N-j)!} \sum_{P, P''} (-1)^{P''} A_{P(1), P'' \circ P(1)}(z) \cdots A_{P(i-1), P'' \circ P(i-1)}(z) \\ &\quad \times \phi_{P(i)}(z) \phi_{P'' \circ P(i)}(z') C_{P(i+1), P'' \circ P(i+1)}(z, z') \cdots C_{P(j), P'' \circ P(j)}(z, z') \\ &\quad \times B_{P(j+1), P'' \circ P(j+1)}(z') \cdots B_{P(N), P'' \circ P(N)}(z') \end{aligned} \quad (51)$$

here, we used

$$(-1)^P (-1)^{P'} = (-1)^P (-1)^{P'' \circ P} = (-1)^P (-1)^{P''} (-1)^P = (-1)^{P''} \quad (52)$$

The ordering among the  $A$ 's,  $B$ 's, and  $C$ 's is irrelevant. Therefore, the sum contains  $(i-1)!(j-i)!(N-j)!$  equal terms. Sum over all decompositions of  $\underline{N}$  into disjoint subsets,  $J + K + L + M = \underline{N}$ , with  $J = \{P(1), \dots, P(i-1)\}$ ,  $K = \{P(i)\}$ ,  $L = \{P(i+1), \dots, P(j)\}$ , and  $M = \{P(j+1), \dots, P(N)\}$ . Multiply by  $(i-1)!(j-i)!(N-j)!$ , since ordering within  $J$ ,  $L$ , and  $M$  is irrelevant

$$\begin{aligned} \rho^{(i,j)}(z, z') &= (-1)^{i+j}\theta(z, z') \sum_{P''} (-1)^{P''} \sum_{J+K+L+M=\underline{N}} \prod_{j \in J} A_{j, P''(j)}(z) \\ &\quad \times \prod_{k \in K} \phi_k(z) \phi_{P''(k)}(z') \prod_{l \in L} C_{l, P''(l)}(z, z') \prod_{m \in M} B_{m, P''(m)}(z'). \end{aligned} \quad (53)$$

Decompose  $J$  into all disjoint subsets  $Q$  and  $R$ ,  $J = Q + R$ .  $P''(q) = q$  for all  $q \in Q$  and  $R = J \setminus Q$ . Then

$$\prod_{j \in J} A_{j, P''(j)}(z) = (-1)^{|J|} \sum_{Q+R=J} (-1)^{|Q|} \prod_{r \in R} B_{r, P''(r)}(z). \quad (54)$$

decompose  $L$  into all disjoint subsets  $S$  and  $T$ ,  $L = S + T$ ; then

$$\begin{aligned} \prod_{l \in L} C_{l, P''(l)}(z, z') &= \prod_{l \in L} [B_{l, P''(l)}(z) - B_{l, P''(l)}(z')] \\ &= \sum_{S+T=L} (-1)^{|T|} \prod_{s \in S} B_{s, P''(s)}(z) \prod_{t \in T} B_{t, P''(t)}(z') \end{aligned} \quad (55)$$

use  $|J| = i-1$ , then

$$\begin{aligned} \rho^{(i,j)}(z, z') &= (-1)^{j+1}\theta(z, z') \sum_{P''} (-1)^{P''} \sum_{Q+R+K+S+T+M=\underline{N}} (-1)^{|Q|+|T|} \prod_{r \in R} B_{r, P''(r)}(z) \\ &\quad \times \prod_{k \in K} \phi_k(z) \phi_{P''(k)}(z') \prod_{s \in S} B_{s, P''(s)}(z) \prod_{t \in T} B_{t, P''(t)}(z') \prod_{m \in M} B_{m, P''(m)}(z') \end{aligned} \quad (56)$$

use

$$\sum_{P'' \in S_N} (-1)^{P''} \sum_{Q+R+K+S+T+M=\underline{N}} \dots = \sum_{Q+R+K+S+T+M=\underline{N}} \sum_{P'' \in S_{\underline{N} \setminus Q}} (-1)^{P''} \dots \quad (57)$$

join  $S$  and  $R$ ,  $U = S + R$ , and  $T$  and  $M$ ,  $V = T + M$ ,

$$\begin{aligned} \rho^{(i,j)}(z, z') &= (-1)^{j+1} \theta(z, z') \sum_{K+Q+U+V=\underline{N}} (-1)^{|Q|+|T|} \binom{|U|}{|S|} \binom{|V|}{|T|} \sum_{P'' \in S_{\underline{N} \setminus Q}} (-1)^{P''} \\ &\quad \times \prod_{k \in K} \phi_k(z) \phi_{P''(k)}(z') \prod_{u \in U} B_{u, P''(u)}(z) \prod_{v \in V} B_{v, P''(v)}(z') \end{aligned} \quad (58)$$

A permutation  $P'' \in S_{K+U+V}$ , either, only permutes the elements of  $U + V$ , or, additionally, it also permutes the one element of  $K$  with one of the elements of  $U + V$ . Therefore

$$\begin{aligned} \rho^{(i,j)}(z, z') &= (-1)^{j+1} \theta(z, z') \sum_{K+Q+U+V=\underline{N}} (-1)^{|Q|+|T|} \binom{|U|}{|S|} \binom{|V|}{|T|} \prod_{k \in K} \phi_k(z) \\ &\quad \times \left\{ \phi_k(z') \sum_{P \in S_{U+V}} (-1)^P \prod_{u \in U} B_{u, P(u)}(z) \prod_{v \in V} B_{v, P(v)}(z') \right. \\ &\quad \left. - \sum_{w \in U+V} \phi_w(z') \sum_{P \in S_{U+V}} (-1)^P \prod_{u \in U} B_{u, P_{k,w} \circ P(u)}(z) \prod_{v \in V} B_{v, P_{k,w} \circ P(v)}(z') \right\}. \end{aligned} \quad (59)$$

Now, we want to sum over  $k \in K$ ,  $l \equiv w \in U + V$ ,  $m \equiv |U|$ , and  $n \equiv |V|$ . Therefore, we express  $|Q|$ ,  $|S|$ , and  $|T|$  by means of  $k$ ,  $l$ ,  $m$ , and  $n$ :

$$|Q| = N - 1 - |U| - |V| = N - 1 - m - n \quad (60)$$

$$|R| = |J| - |Q| = i - 1 - (N - 1 - m - n) = i - N + m + n \quad (61)$$

$$|S| = |U| - |R| = m - (i - N + m + n) = N - i - n \quad (62)$$

$$|T| = |L| - |S| = j - i - (N - i - n) = j - N + n. \quad (63)$$

Therefore

$$(-1)^{j+1} (-1)^{|Q|+|T|} = (-1)^{j+1} (-1)^{j-1-m} = (-1)^m. \quad (64)$$

Which values can  $k$ ,  $l$ ,  $m$ , and  $n$  assume?  $k$  can assume the values  $1, \dots, N$ , i.e.  $k = 1, \dots, N$ .  $l$  cannot assume the value  $k$ , since  $K \cap (U + V) = \emptyset$ . Therefore  $l = 1, \dots, N$ , but  $l \neq k$ .  $m = |U| = |S| + |R|$  can assume the values  $0, \dots, j - 1$ , since  $|S| = 0, \dots, |L| = j - i$  and  $|R| = 0, \dots, |J| = i - 1$ , i.e.  $m = 0, \dots, j - 1$ .

$$\begin{aligned} n &= |V| = |M| + |T| = N - j + |T| = N - j + |L| - |S| = N - j + j - i - |S| \\ &= N - i - |S| \end{aligned} \quad (65)$$

Therefore  $n = N - j, \dots, N - i$ , since  $|S| = 0, \dots, |L| = j - i$ . Moreover, we have to take into account that  $|U| + |V| \leq N - 1$  and  $|S| \leq |U|$ , which leads to the inequalities  $n \leq N - m - 1$



and  $n \geq N - i - m$ , respectively. Therefore  $n = N - \min(j, m + i), \dots, N - \max(i, m + 1)$ . We obtain in the next step

$$\begin{aligned}
\rho^{(i,j)}(z, z') &= \theta(z, z') \sum_{k=1}^N \sum_{m=0}^{j-1} \sum_{n=N-\min(j, m+i)}^{N-\max(i, m+1)} \phi_k(z) \phi_k(z') \\
&\quad \times (-1)^m \binom{m}{N-i-n} \binom{n}{j-N+n} \sum_{p \in P(k, k, m, n)} \det B_p \\
&\quad - \theta(z, z') \sum_{k=1}^N \sum_{l \neq k=1}^N \sum_{m=0}^{j-1} \sum_{n=N-\min(j, m+i)}^{N-\max(i, m+1)} \phi_k(z) \phi_l(z') \\
&\quad \times (-1)^m \binom{m}{N-i-n} \binom{n}{j-N+n} \sum_{p \in P(k, l, m, n)} \det B_p. \tag{66}
\end{aligned}$$

$P(k, k, m, n)$  is the set of pairs of ordered  $m$ - and  $n$ -tuples  $p = (i_1, \dots, i_m)(j_1, \dots, j_n)$  with  $\{i_1, \dots, i_m\}, \{j_1, \dots, j_n\} \subset \underline{N} \setminus \{k\}$ , and  $\{i_1, \dots, i_m\} \cap \{j_1, \dots, j_n\} = \emptyset$ .  $p$  are the row and column indices of  $B_p$ .  $(i_1, \dots, i_m)$  and  $(j_1, \dots, j_n)$  are the row indices of matrix elements  $B_{i,j}(z)$  and  $B_{i,j}(z')$ , respectively.  $P(k, l, m, n)$  is the set of pairs of ordered  $m$ - and  $n$ -tuples  $p = (i_1, \dots, i_m)(j_1, \dots, j_n)$  with disjoint sets  $\{i_1, \dots, i_m\}$  and  $\{j_1, \dots, j_n\}$ , which contain elements of  $\underline{N} \setminus \{k, l\}$  and where one of the sets also contains the element  $l$ . The column indices  $\bar{p}$  are obtained from  $p$  by replacing  $l$  by  $k$ . Additionally we define

$$\sum_{p \in P(k, l, 0, 0)} \det B_p = \delta_{k, l}. \tag{67}$$

Finally, we obtain

$$\begin{aligned}
\rho^{(i,j)}(z, z') &= \theta(z, z') \sum_{k, l=1}^N \sum_{m=0}^{j-1} \sum_{n=N-\min(j, m+i)}^{N-\max(i, m+1)} (2\delta_{k, l} - 1) \phi_k(z) \phi_l(z') \\
&\quad \times (-1)^m \binom{m}{N-i-n} \binom{n}{j-N+n} \sum_{p \in P(k, l, m, n)} \det B_p. \tag{68}
\end{aligned}$$

The analog formula with  $A$ -matrices reads

$$\begin{aligned}
\rho^{(i,j)}(z, z') &= \theta(z, z') \sum_{k, l=1}^N \sum_{m=i-1}^{j-1} \sum_{n=j-m-1}^{N-i} (2\delta_{k, l} - 1) \phi_k(z) \phi_l(z') \\
&\quad \times (-1)^n \binom{m}{m+1-i} \binom{n}{j-m-1} \sum_{p \in P(k, l, m, n)} \det A_p. \tag{69}
\end{aligned}$$
